# Supplementary material for: Brightened Optical Transition as Indicator of Multiferroicity in a Layered Antiferromagnet
Source: arXiv:2405.17144 ancillary file (2024-05-27)
Supplement: Supplementary file 1 [file sm.pdf]

# Brightened Optical Transition as Indicator of Multiferroicity in a Layered Antiferromagnet

Volodymyr Multian,[1,2,3] Fan Wu,[1,2] Dirk van der Marel,[1] Nicolas Ubrig,[1] and Jérémie Teyssier[1]

[1] *Department of Quantum Matter Physics, University of Geneva, 24 Quai Ernest Ansermet, CH-1211 Geneva, Switzerland*

[2] *Department of Applied Physics, University of Geneva, 24 Quai Ernest Ansermet, CH-1211 Geneva, Switzerland*

[3] *Advanced Materials Nonlinear Optical Diagnostics lab, Institute of Physics, NAS of Ukraine, 46 Nauky pr., 03028, Kyiv, Ukraine*

## CONTENTS

I. Methods 2

II. Eigenstates of the 3d orbital states 3

III. References 5

## I. METHODS

### Raman, photoluminescence and Second Harmonic Generation measurement

Raman, photoluminescence (PL) and Second Harmonic Generation (SHG) measurements are performed on a unique instrument. We coupled a pulsed Ti:Saphire laser (Coherent Vitesse 800 nm, 100 fs, 80 MHz) to a commercial Raman spectrometer (Horiba LabRAM HR Evolution) using a patented optical module[1] allowing simultaneous recording of polarisation resolved Raman, PL and SHG signals. A mm-size bulk $CrPS_4$ crystal is glued (silver paint) on the cold finger of a He flow cryostat (Konti Micro from CryoVac GmbH) allowing measurements from 4K to 350K. Raman and PL spectra are acquired in confocal configuration with a spectral resolution of 0.3 $cm^{-1}$ (0.04 meV). Laser beams from continuous wave lasers emitting at 405 nm or 532 nm and ultrafast laser at 800 nm are focused on the same spot with sizes ranging from 0.4 to 1.0 $\mu$m (FWHM) with window-corrected 63$\times$ objective. For Raman/PL excitation lasers, a home-tailored module based on a set of the quarter wave (ThorLabs AQWP05M-600) and half wave (ThorLabs AHWP05M-600) plates mounted in motorized stages is used for continuously tune the polarization from linear to circular. Analysis of the polarization state of Raman and PL signals is achieved placing a Glan-Laser polarizer (ThorLabs GL10, extinction ratio 100 000:1) mounted in the motorized rotation stage, followed by a depolarizer (ThorLabs DPP25-A), at the entrance of the spectrometer. Signal acquisition was performed with LN cooled Si charge coupled device (CCD) array (Horiba Scientific Symphony II). The laser power is set to 0.2 $\mu$W to minimize the effect of laser heating. The temperature of the sample at the laser spot is corrected using Raman Stokes/anti-Stokes ratio as implemented in Reffit program[2,3].

SHG signal at 400 nm is collected in epidetection geometry in a separate optical channel using a LN-cooled CCD array (Princeton Instruments). A cascade of 3 band-pass interference filters rejects the excitation laser light (ThorLabs FBH400-10, CWL = 400 nm, FWHM = 10 nm ). The angle of linear polarization of the incident beam is optimized to maximize the SHG signal. The signal acquisition is realized in a parallel configuration to the incidence polarization with the use of a Glan-Thompson polarizer (ThorLabs GTH10M) in front of the CCD. The average power of pump beam is set to 10 mW which corresponds to peak power density of 150 GW/cm$^2$. The laser heating is again estimated by Raman-based thermometry performed from the same spot.

**Photocurrent.** Photocurrent measurements were performed by illuminating the sample with a supercontinuum white light laser passing through a contrast filter, allowing the laser wavelength to be tuned continuously between 400 and 1100 nm, while keeping the power fixed at 50 $\mu$W. For these measurements, the sample was placed in the cryostat on a holder mounted on a piezo-electric driven x-y stage, allowing stepping the position of the sample relative to the beam with a precision of 50 nm (Cryovac KONTI). The photocurrent was then measured with home-made low noise voltage and current amplifiers, and read out by digital multimeters. For the photocurrent measurements we fabricated thin layered samples (about 10 nm thickness) with thin graphite electrodes following the procedure described in References[4].

## II. EIGENSTATES OF THE 3d ORBITAL STATES

In the main text figure 3d we sketch the orbital occupation of the ground and excited states of the $Cr^{3+}$. For the sake of completeness we discuss the nature of their eigenstates. The spectroscopic notation $^{2S+1}X_j$ used here characterizes the many-body eigenstates of the 3 electrons in the $Cr^{3+}$ $3d$-shell in terms of the quantum numbers. For example, if the spins of the 3 electrons are all parallel to each other, their total spin is $S = 3/2$ and the $m_S$ can be $\pm 3/2$ or $\pm 1/2$, amounting to $2S + 1 = 4$ different eigenstates with the same energy. The labels $A$, $E$, $T$ indicate the orbital character of the $3d^3$ many-body state. For $A$ there is 1 such state, for $E$ there are 2 and for $T$ 3 degenerate states. The eigenstates for the most relevant many-body states are provided.

In an octahedral environment with infinite crystal field, the only available orbitals are $d_{xy}$, $d_{yz}$ and $d_{zx}$. For a system with 3 electrons, in the ground state each electron will occupy a different orbital, and each can have spin up or spin down providing $2 \times 2 \times 2 = 8$ possible configurations. The lowest interaction energy is obtained if the total spin of the electrons is maximal, in the present case $S = 3/2$, providing 4 different spin states. Consequently the

ground state is one of the four $^4A$ states, or a linear combination thereof:

$$
\begin{aligned}
|g\rangle &= \sum_{m=-3/2}^{3/2} \alpha_m |^4A_2; m\rangle \\
|^4A_2; 3/2\rangle &= d^\dagger_{xy\uparrow}, d^\dagger_{yz\uparrow}, d^\dagger_{zx\uparrow}|0\rangle \\
|^4A_2; 1/2\rangle &= \sqrt{1/3}\{d^\dagger_{xy\downarrow}, d^\dagger_{yz\uparrow}, d^\dagger_{zx\uparrow} + d^\dagger_{xy\uparrow}, d^\dagger_{yz\downarrow}, d^\dagger_{zx\uparrow} + d^\dagger_{xy\uparrow}, d^\dagger_{yz\uparrow}, d^\dagger_{zx\downarrow}\}|0\rangle \\
|^4A_2; -1/2\rangle &= \sqrt{1/3}\{d^\dagger_{xy\uparrow}, d^\dagger_{yz\downarrow}, d^\dagger_{zx\downarrow} + d^\dagger_{xy\downarrow}, d^\dagger_{yz\uparrow}, d^\dagger_{zx\downarrow} + d^\dagger_{xy\downarrow}, d^\dagger_{yz\downarrow}, d^\dagger_{zx\uparrow}\}|0\rangle \\
|^4A_2; -3/2\rangle &= d^\dagger_{xy\downarrow}, d^\dagger_{yz\downarrow}, d^\dagger_{zx\downarrow}|0\rangle
\end{aligned}
\tag{1}
$$

If the total spin is 1/2, the interaction energy is higher than in the ground state. This extra interaction amounts to $9B + 3C \sim 2$ eV where $B$ and $C$ are Racah parameters. The corresponding set of eigenstates is

$$
\begin{aligned}
|^2E; +, \uparrow\rangle &= \sqrt{1/3}\{d^\dagger_{xy\downarrow}, d^\dagger_{yz\uparrow}, d^\dagger_{zx\uparrow} + e^{i2\pi/3} d^\dagger_{xy\uparrow}, d^\dagger_{yz\downarrow}, d^\dagger_{zx\uparrow} + e^{i4\pi/3} d^\dagger_{xy\uparrow}, d^\dagger_{yz\uparrow}, d^\dagger_{zx\downarrow}\}|0\rangle \\
|^2E; -, \uparrow\rangle &= \sqrt{1/3}\{d^\dagger_{xy\downarrow}, d^\dagger_{yz\uparrow}, d^\dagger_{zx\uparrow} + e^{-i2\pi/3} d^\dagger_{xy\uparrow}, d^\dagger_{yz\downarrow}, d^\dagger_{zx\uparrow} + e^{-i4\pi/3} d^\dagger_{xy\uparrow}, d^\dagger_{yz\uparrow}, d^\dagger_{zx\downarrow}\}|0\rangle \\
|^2E; +, \downarrow\rangle &= \sqrt{1/3}\{d^\dagger_{xy\uparrow}, d^\dagger_{yz\downarrow}, d^\dagger_{zx\downarrow} + e^{i2\pi/3} d^\dagger_{xy\downarrow}, d^\dagger_{yz\uparrow}, d^\dagger_{zx\downarrow} + e^{i4\pi/3} d^\dagger_{xy\downarrow}, d^\dagger_{yz\uparrow}, d^\dagger_{zx\downarrow}\}|0\rangle \\
|^2E; -, \downarrow\rangle &= \sqrt{1/3}\{d^\dagger_{xy\uparrow}, d^\dagger_{yz\downarrow}, d^\dagger_{zx\downarrow} + e^{-i2\pi/3} d^\dagger_{xy\downarrow}, d^\dagger_{yz\uparrow}, d^\dagger_{zx\downarrow} + e^{-i4\pi/3} d^\dagger_{xy\downarrow}, d^\dagger_{yz\uparrow}, d^\dagger_{zx\downarrow}\}|0\rangle
\end{aligned}
\tag{2}
$$

In total there exist 20 states where 3 electrons occupy the three $d_{xy}$, $d_{yz}$ and $d_{zx}$ orbitals. Together $^4A$ and $^2E$ form the subset of states where each these three orbitals is occupied by precisely 1 electron. The other 12 states have one of the three orbitals empty, one occupied with a single electron and one with 2 electrons of opposite spin. They are grouped in two 6-fold degenerate manifolds labeled $^2T_1$ (energy $E_g + 9B + 3C$)

$$
\begin{aligned}
|^2T_1; yz, \uparrow\rangle &= \sqrt{1/2}\{d^\dagger_{yz\uparrow}, d^\dagger_{zx\uparrow}, d^\dagger_{zx\downarrow} + d^\dagger_{yz\uparrow}, d^\dagger_{xy\uparrow}, d^\dagger_{xy\downarrow}\}|0\rangle \\
|^2T_1; zx, \uparrow\rangle &= \sqrt{1/2}\{d^\dagger_{xy\uparrow}, d^\dagger_{yz\uparrow}, d^\dagger_{yz\downarrow} + d^\dagger_{xy\uparrow}, d^\dagger_{zx\uparrow}, d^\dagger_{zx\downarrow}\}|0\rangle \\
|^2T_1; xz, \uparrow\rangle &= \sqrt{1/2}\{d^\dagger_{zx\uparrow}, d^\dagger_{xy\uparrow}, d^\dagger_{xy\downarrow} + d^\dagger_{zx\uparrow}, d^\dagger_{yz\uparrow}, d^\dagger_{xz\downarrow}\}|0\rangle \\
|^2T_1; yz, \downarrow\rangle &= \sqrt{1/2}\{d^\dagger_{yz\downarrow}, d^\dagger_{zx\uparrow}, d^\dagger_{zx\downarrow} + d^\dagger_{yz\downarrow}, d^\dagger_{xy\uparrow}, d^\dagger_{xy\downarrow}\}|0\rangle \\
|^2T_1; zx, \downarrow\rangle &= \sqrt{1/2}\{d^\dagger_{xy\downarrow}, d^\dagger_{yz\uparrow}, d^\dagger_{yz\downarrow} + d^\dagger_{xy\downarrow}, d^\dagger_{zx\uparrow}, d^\dagger_{zx\downarrow}\}|0\rangle \\
|^2T_1; xy, \downarrow\rangle &= \sqrt{1/2}\{d^\dagger_{zx\downarrow}, d^\dagger_{xy\uparrow}, d^\dagger_{xy\downarrow} + d^\dagger_{zx\downarrow}, d^\dagger_{yz\uparrow}, d^\dagger_{xz\downarrow}\}|0\rangle
\end{aligned}
$$

and $^2T_2$ (energy $E_g + 15B + 5C$)

$$
\begin{aligned}
|^2T_2; yz, \uparrow\rangle &= \sqrt{1/2}\{d^\dagger_{yz\uparrow}, d^\dagger_{zx\uparrow}, d^\dagger_{zx\downarrow} - d^\dagger_{yz\uparrow}, d^\dagger_{xy\uparrow}, d^\dagger_{xy\downarrow}\}|0\rangle \\
|^2T_2; zx, \uparrow\rangle &= \sqrt{1/2}\{d^\dagger_{xy\uparrow}, d^\dagger_{yz\uparrow}, d^\dagger_{yz\downarrow} - d^\dagger_{xy\uparrow}, d^\dagger_{zx\uparrow}, d^\dagger_{zx\downarrow}\}|0\rangle \\
|^2T_2; xy, \uparrow\rangle &= \sqrt{1/2}\{d^\dagger_{zx\uparrow}, d^\dagger_{xy\uparrow}, d^\dagger_{xy\downarrow} - d^\dagger_{zx\uparrow}, d^\dagger_{yz\uparrow}, d^\dagger_{xz\downarrow}\}|0\rangle \\
|^2T_2; yz, \downarrow\rangle &= \sqrt{1/2}\{d^\dagger_{yz\downarrow}, d^\dagger_{zx\uparrow}, d^\dagger_{zx\downarrow} - d^\dagger_{yz\downarrow}, d^\dagger_{xy\uparrow}, d^\dagger_{xy\downarrow}\}|0\rangle \\
|^2T_2; zx, \downarrow\rangle &= \sqrt{1/2}\{d^\dagger_{xy\downarrow}, d^\dagger_{yz\uparrow}, d^\dagger_{yz\downarrow} - d^\dagger_{xy\downarrow}, d^\dagger_{zx\uparrow}, d^\dagger_{zx\downarrow}\}|0\rangle \\
|^2T_2; xy, \downarrow\rangle &= \sqrt{1/2}\{d^\dagger_{zx\downarrow}, d^\dagger_{xy\uparrow}, d^\dagger_{xy\downarrow} - d^\dagger_{zx\downarrow}, d^\dagger_{yz\uparrow}, d^\dagger_{xz\downarrow}\}|0\rangle
\end{aligned} \tag{3}
$$

We finally mention that the $^4T_1$ and $^4T_2$ states have 2 electrons in the one of the $d_{xy}$, $d_{yz}$ and $d_{zx}$ orbitals, and 1 electron in $d_{z^2}$ or $d_{x^2-y^2}$. The excitation from $^4A$ to $^4T_1$ or $^4T_2$ therefore has to overcome the crystal field splitting, in the present case about 1.35 eV.

## III. REFERENCES


[1] V. Multian and J. Teyssier, "A beam splitting/mixing module for an optical system and an associated optical system," Patent Pending.

[2] I. Ardizzone, J. Teyssier, I. Crassee, A. B. Kuzmenko, D. G. Mazzone, D. J. Gawryluk, M. Medarde, and D. van der Marel, Physical Review Research **3**, 033007 (2021), publisher: American Physical Society.

[3] A. B. Kuzmenko, Review of Scientific Instruments **76**, 083108 (2005).

[4] F. Wu, M. Gibertini, K. Watanabe, T. Taniguchi, I. Gutiérrez-Lezama, N. Ubrig, and A. F. Morpurgo, Advanced Materials **35**, 2211653 (2023), _eprint: https://onlinelibrary.wiley.com/doi/pdf/10.1002/adma.202211653.
